# Supplementary material for: The role of the Big Geographic Sort in the circulation of misinformation among U.S. Reddit users
Source: arXiv:2205.10161 source file (2022-05-20)
Supplement: Supplementary file 1 [file appendix.tex]

\section*{Data}

\subsection*{Reddit User Representativeness}
In this section, we included additional analysis focused on the representativeness of Reddit users with respect to party affiliation. Results are summarized on Figure~\ref{fig:statecorr1} and Figure~\ref{fig:statecorr2}. For Figure~\ref{fig:statecorr1}, the x-axis is calculated as the percentage of population leaning Republican minus percentage of population leaning Democrat. The y-axis is the Reddit adoption rate which was calculated as the number of Reddit users from a given state divided by the state's population. As shown, democratic-leaning states had a significantly higher adoption rate than Republican-leaning states. Next, we also computed the average number of Reddit comments by users from each state and plotted the result against each state's political affiliation. As shown in Figure~\ref{fig:statecorr2}, users from Democratic-leaning states contributed more comments on average than Republican-leaning states. Results suggest that Democratic-leaning states are over-represented compared to Republican-leaning states due to having more users present on Reddit and also the users being more active.

\begin{figure}[hptb]
\centering
\begin{subfigure}{0.5\textwidth}
    \includegraphics[width=0.8\linewidth]{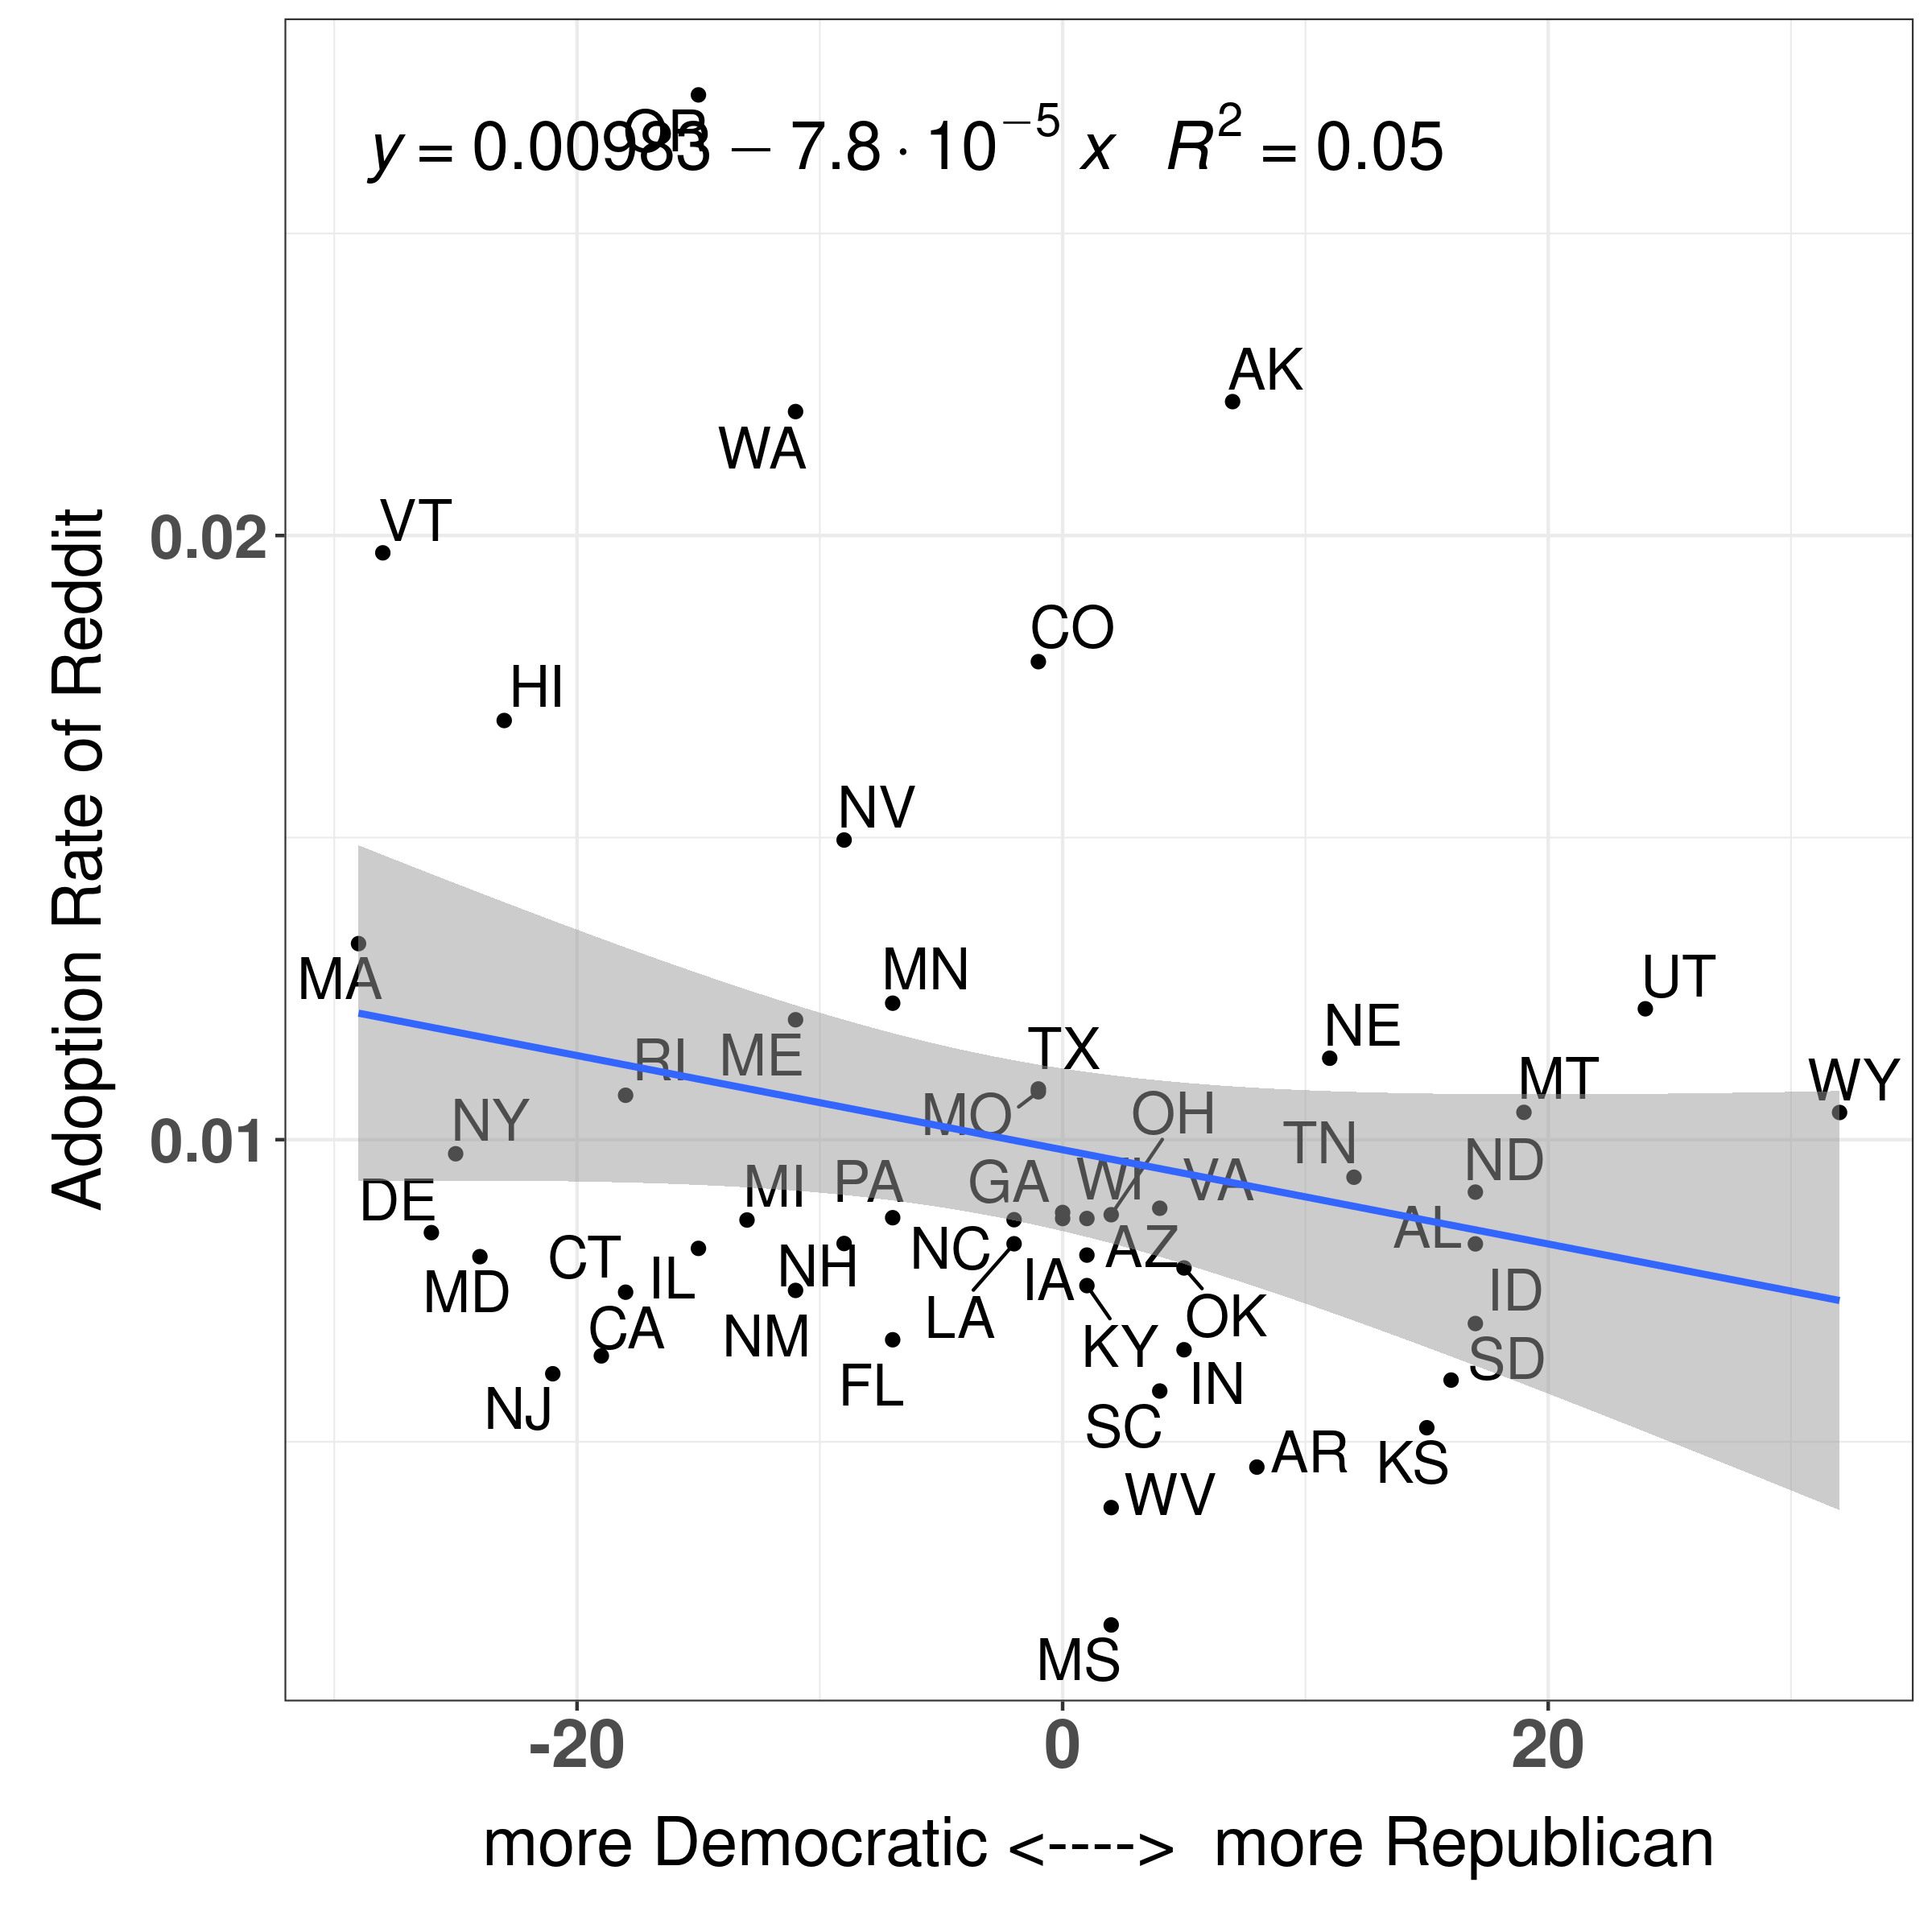}
    \caption{Correlation between state's political leaning and its Reddit adoption rate.}
    \label{fig:statecorr1}
\end{subfigure}%
\begin{subfigure}{0.5\textwidth}
    \includegraphics[width=.8\linewidth]{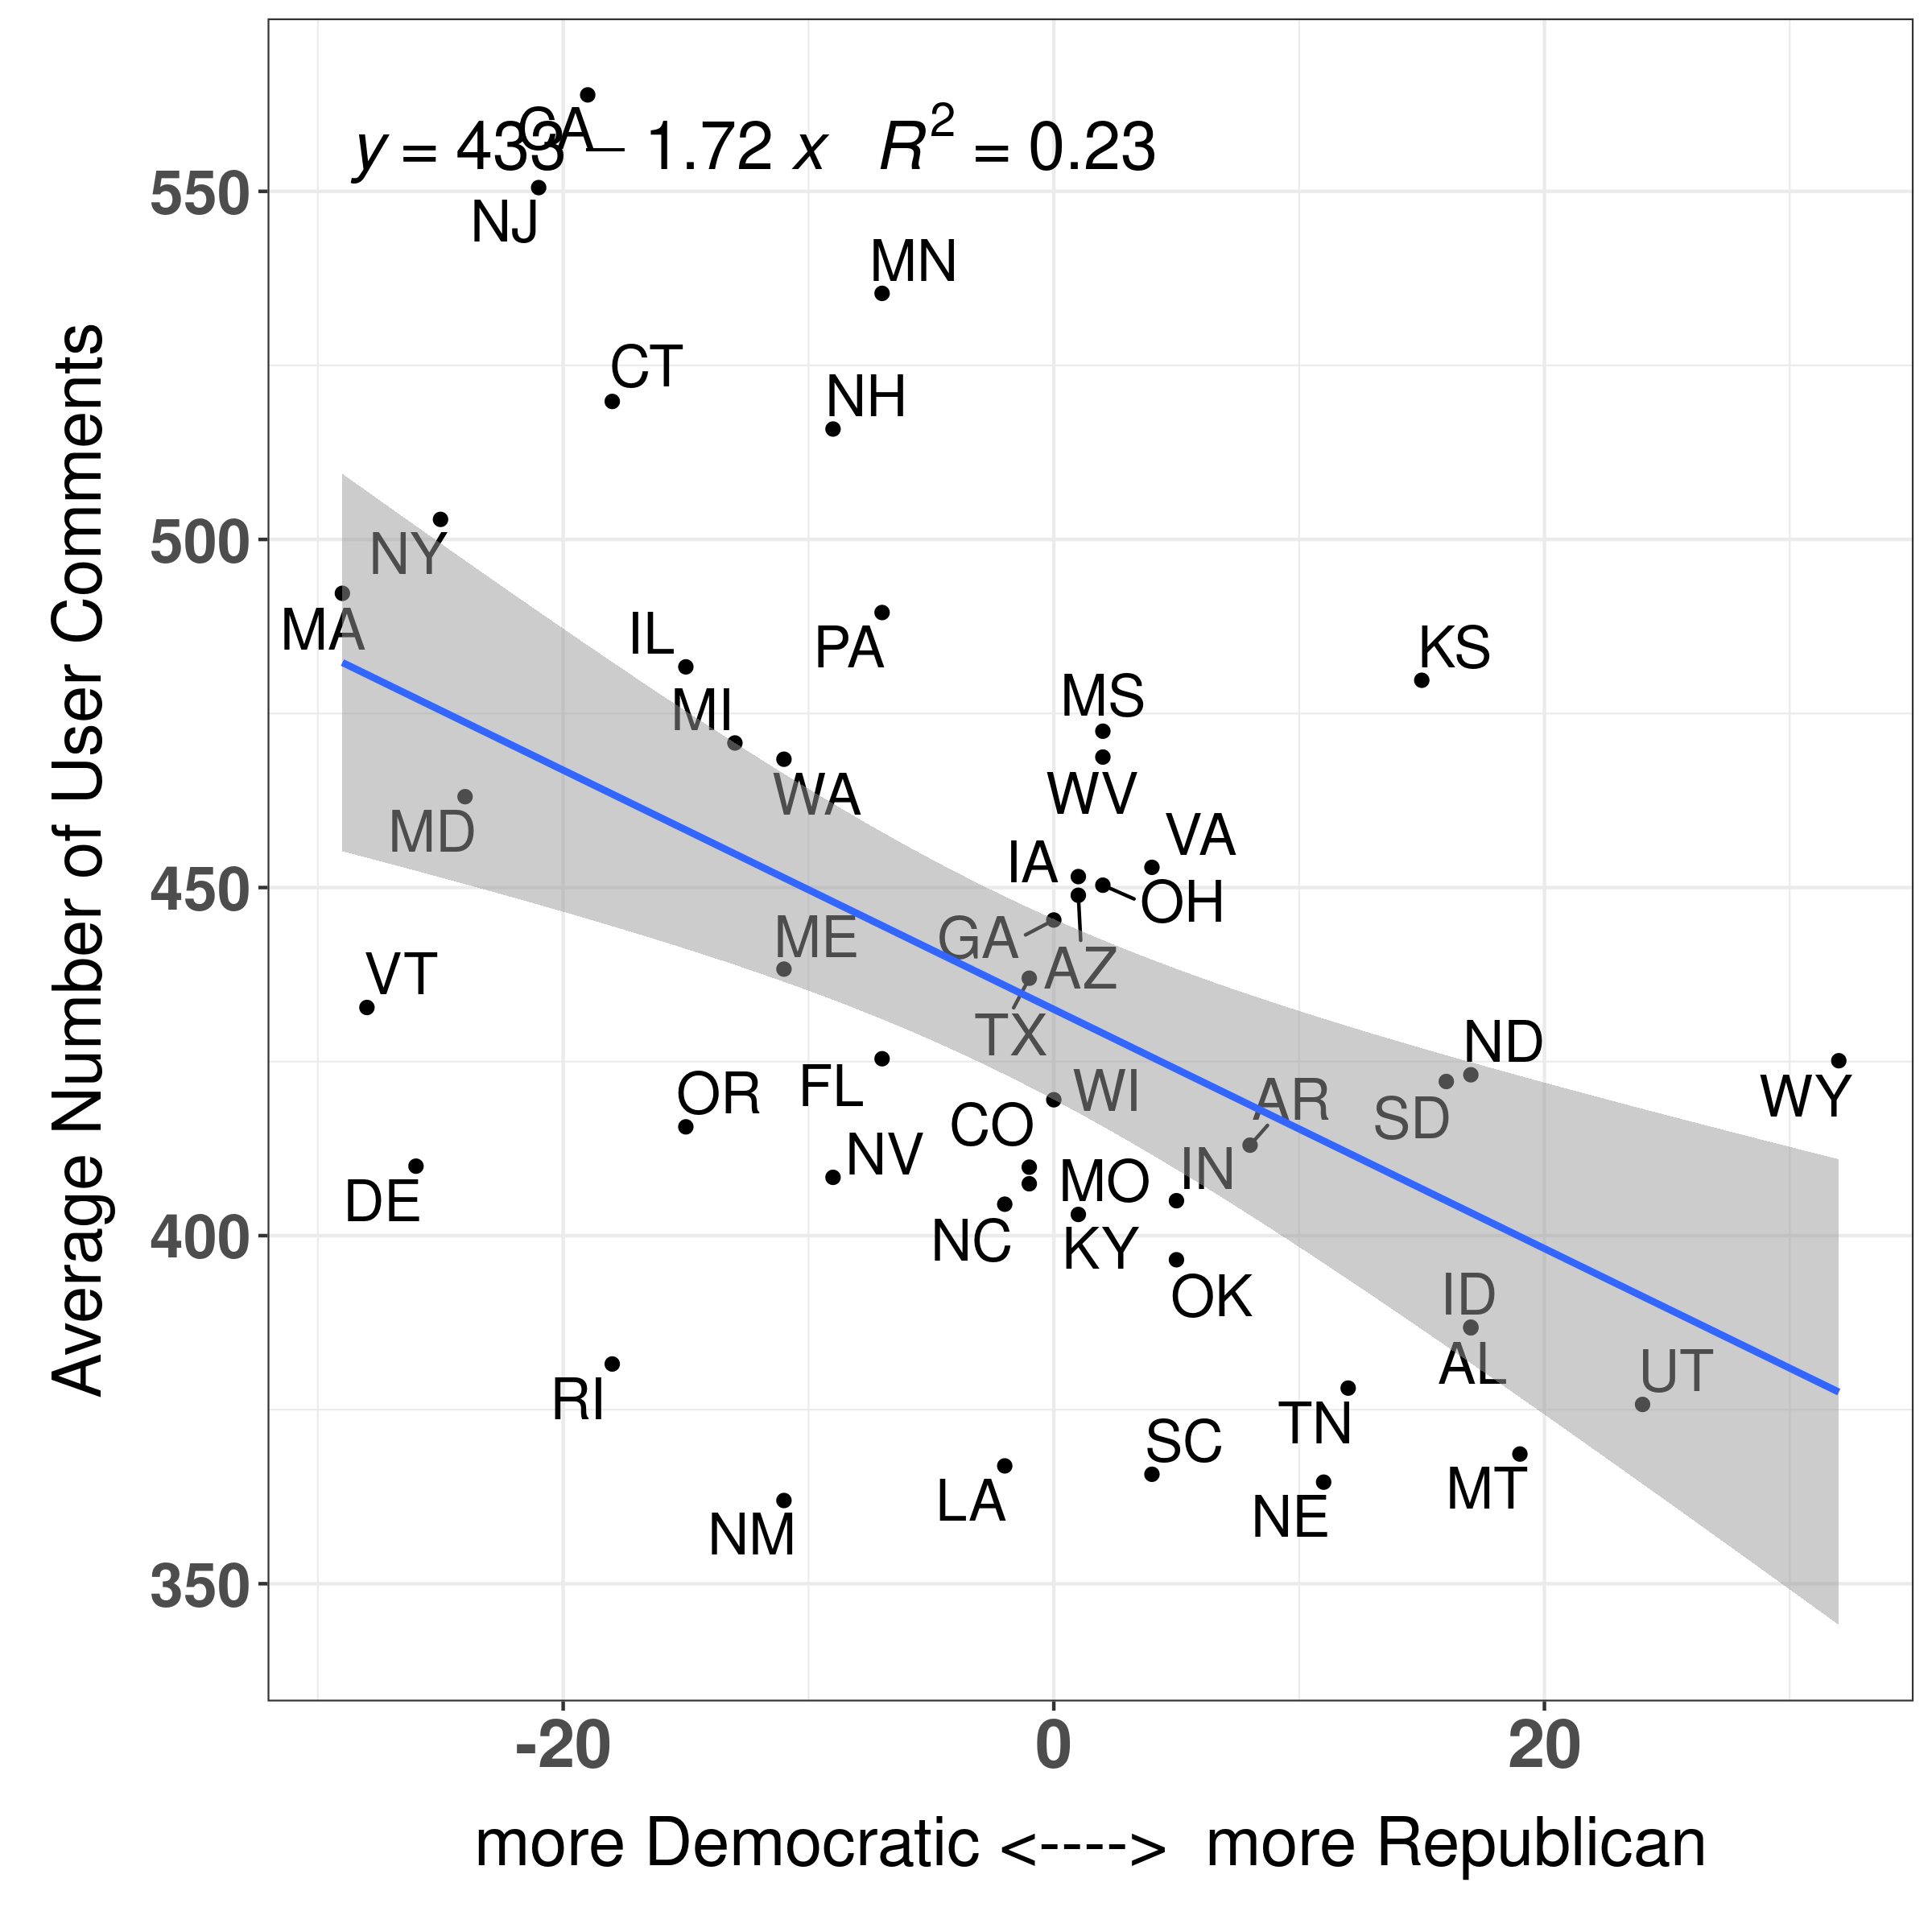}
    \caption{Correlation between state's political leaning and its Reddit activity level.}
    \label{fig:statecorr2}
\end{subfigure}
\label{fig:statecorr}
\caption{Reddit Data Representativeness}
\end{figure}

\subsection*{Geotagged Users VS. Non-geotagged Users}
\begin{figure}[hptb]
    \centering
    \includegraphics[width=0.8\linewidth]{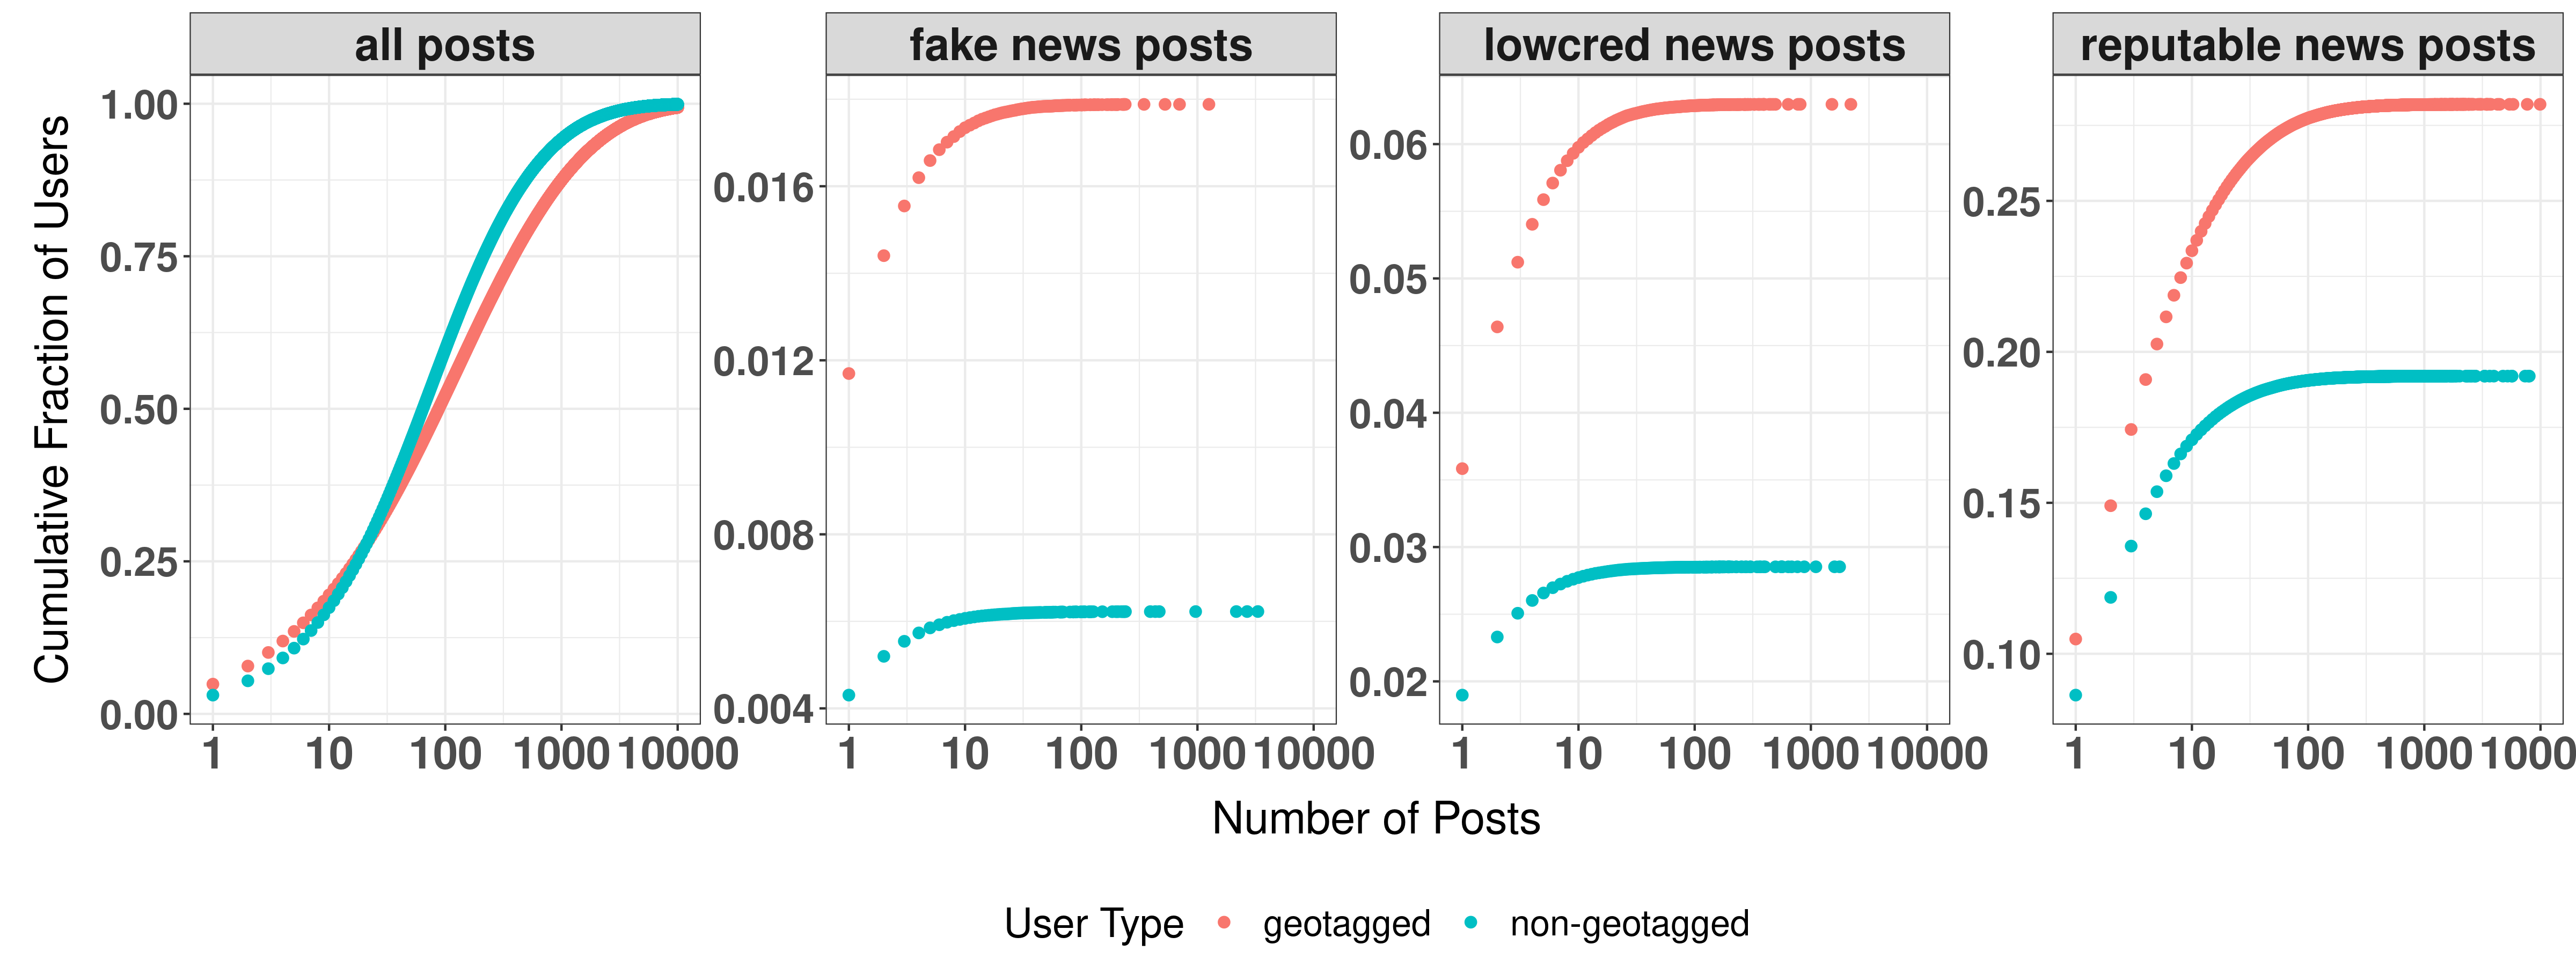}
    \caption{Comparing Geotagged and Non-geotagged Users. We saw that users are comparable in terms of overall comments. However, geotagged users posted more news comments. For instance, approximately 30\% of all geotagged users had posted at least 1 comment containing URLs from reputable news sites. In comparison, only 20\% of non-geotagged users did.}
    \label{fig:user_compare}
\end{figure}
We first sampled approximately 3 million users that were not matched to one of the 50 U.S. states. We then compared the Reddit activity levels of these non-geotagged users to the set of geotagged users (those that were assigned to to one of the U.S. states). We observed that the numbers of total Reddit comments posted by users of the two groups are comparable. Specifically, an average geotagged user posted a total of 88 comments and an average non-geotagged user posted 65 comments. However, we also saw that geotagged users had higher numbers of news comments. For instance, 1.7\% of all geotagged users had posted at least 1 comment containing fake news URLs, whereas only 0.6\% of non-geotagged users did. Similarly, 28.2\% of all geotagged users had posted at least 1 comment containing reputable news URLs, but only 19.2\% of non-geotagged users did. Results are shown in Figure~\ref{fig:user_compare}. The difference here can be explained by non-geotagged users being less likely to be from the U.S., and thus less invested in the ongoing of the U.S..

\subsection*{Groundtruth Labels Robustness Check} 
Here, we compared our news categorization ({\it fake, lowcred} and {\it reputable}) to the trustworthiness scores provided by related work~\cite{pennycook2019fighting}. Specifically, Pennycook et al.~\cite{pennycook2019fighting} provided a list of 60 news sites with trustworthiness ratings ($0-100$ where 100 is completely trustworthy) from professional fact checkers. As shown in Figure~\ref{fig:trustworthy}, of the 60 news sites, those labeled as reputable in our paper had the highest trustworthiness scores (average score was 0.66), followed by those labeled as low-credibility (average score was 0.1) and then fake news sites (average score was 0.02). Results here indicate that our classification labeling is aligned with the ratings by professional fact checkers.

\begin{figure}[hptb]
    \centering
    \includegraphics[width=0.33\linewidth]{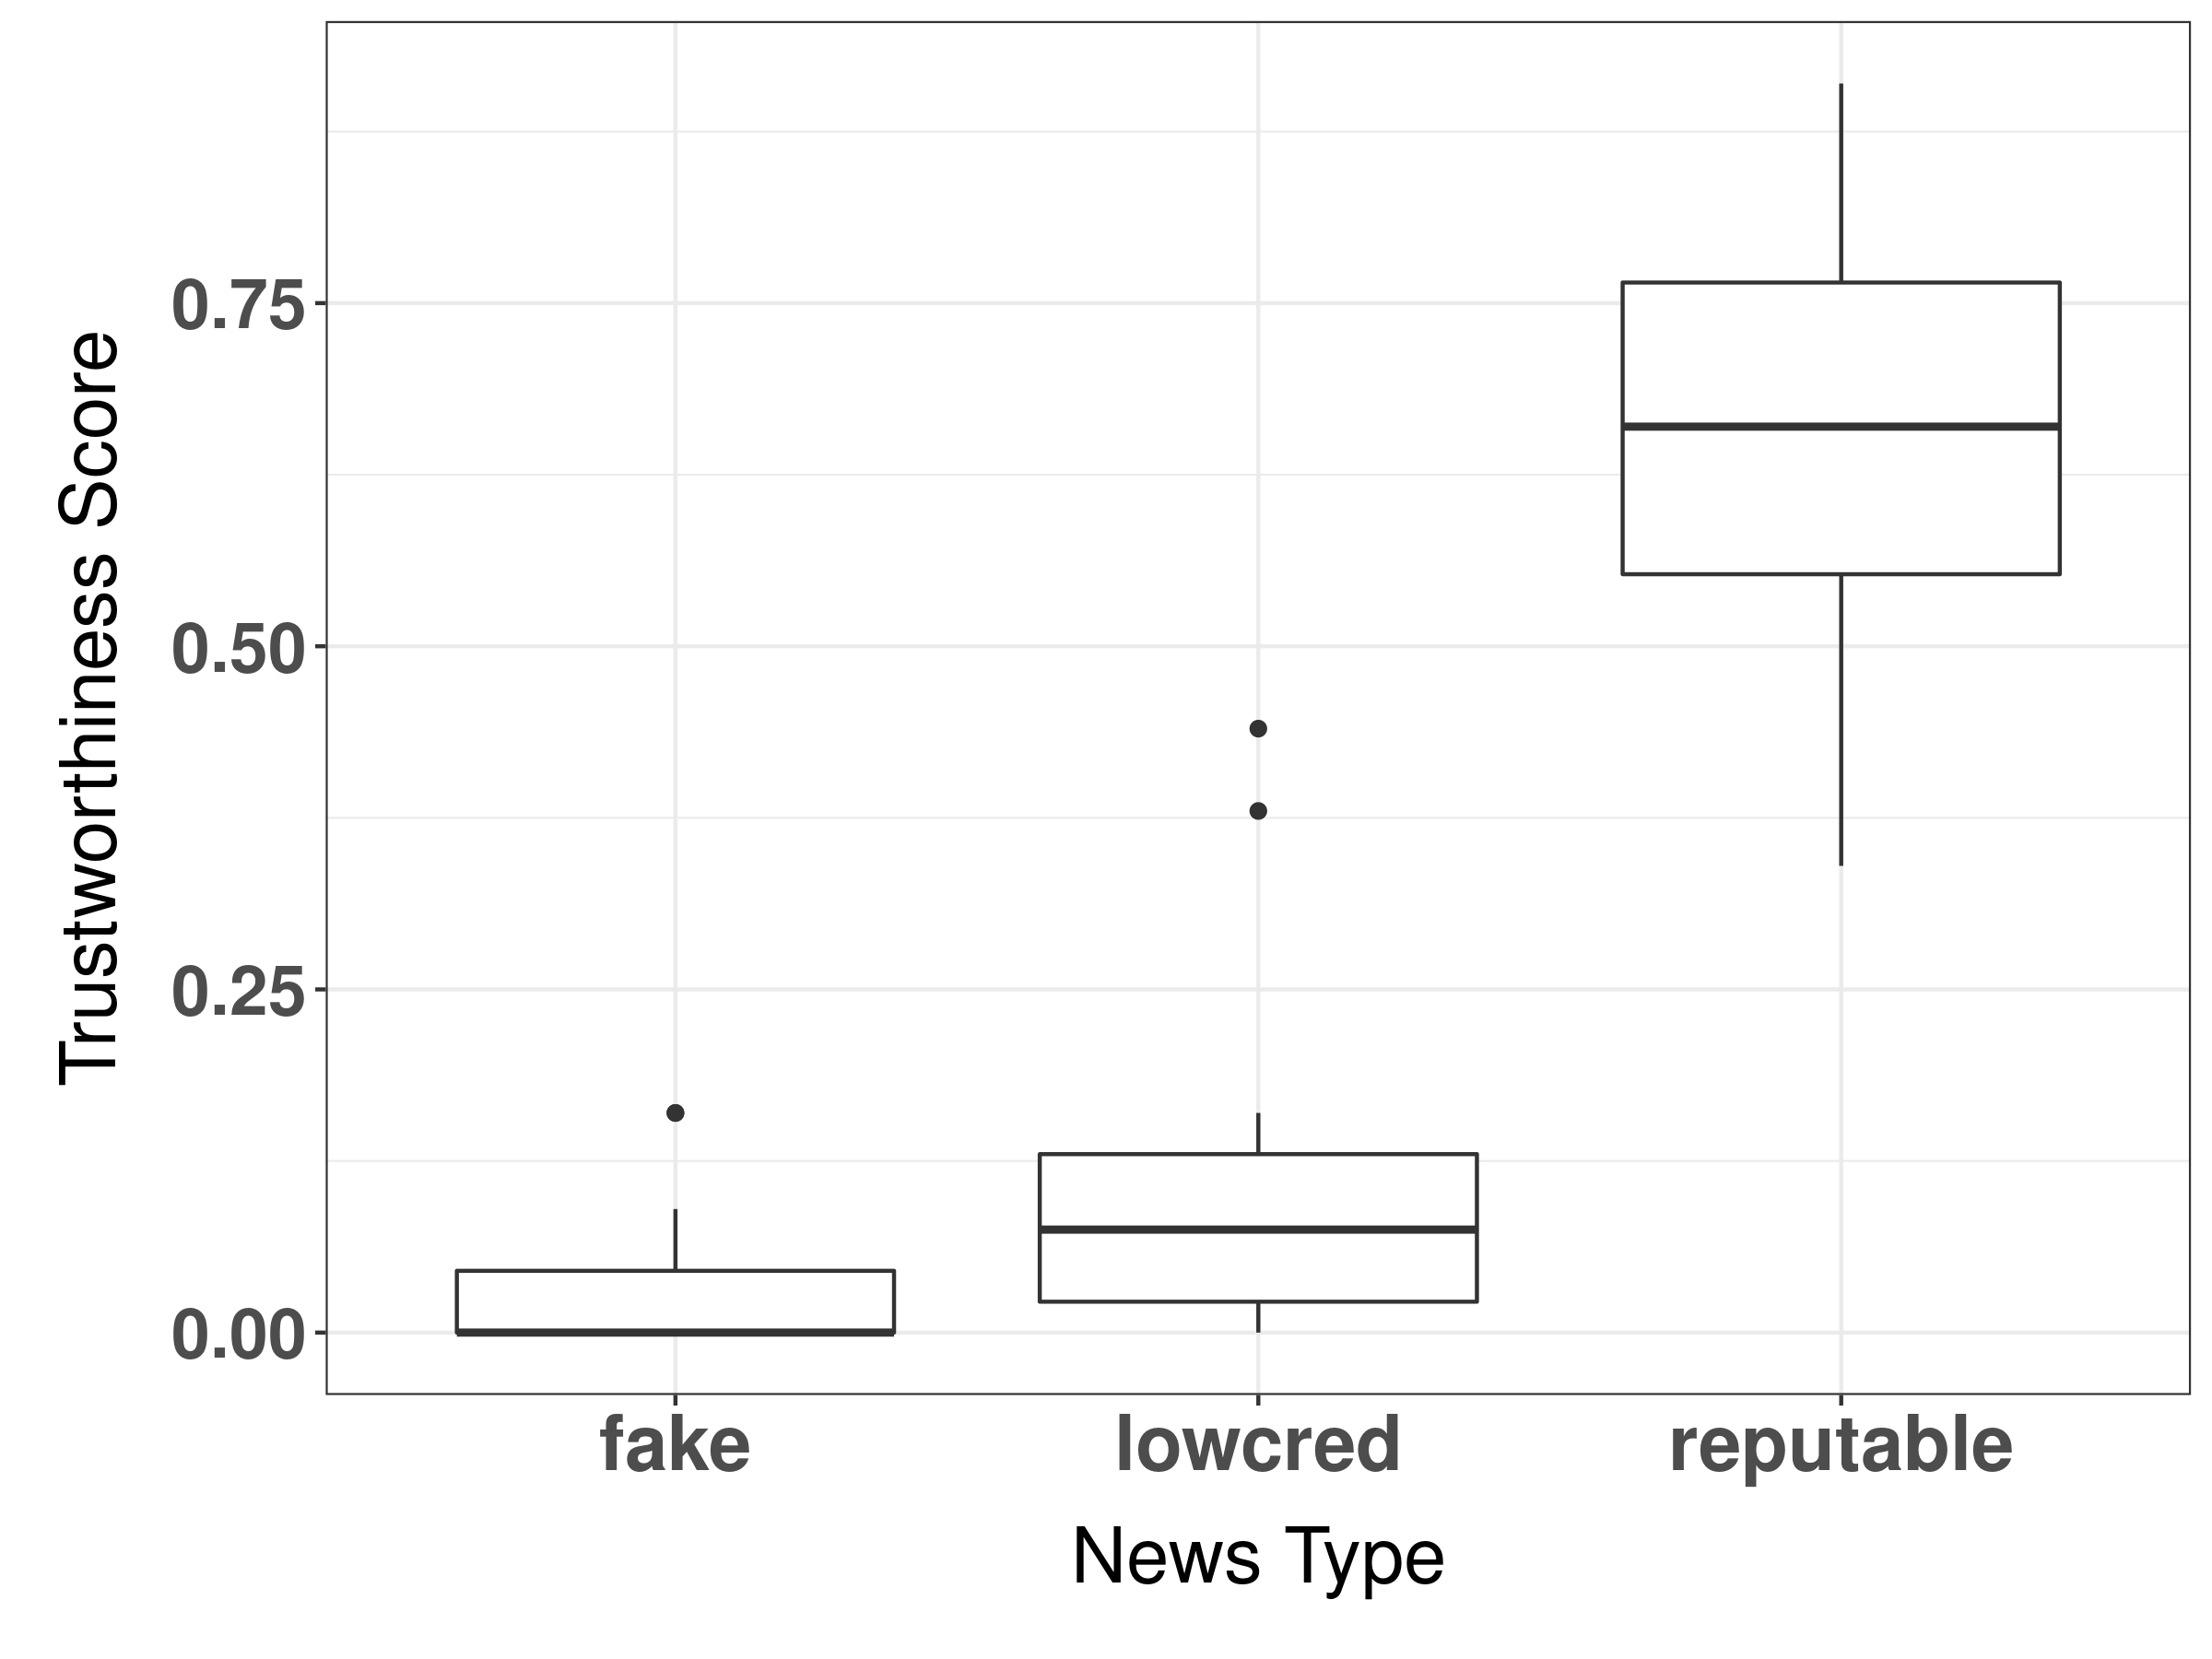}
    \caption{The distribution of trustworthiness scores for each news type.}
    \label{fig:trustworthy}
\end{figure}

\section*{Results}
\subsection*{Geographical Segregation on Facebook} 
We compared the extent of Reddit users' geographical segregation to that of Facebook's. We use the Social Connectivity Index (SCI) of states from Bailey et al.~\cite{bailey2018social}. The SCI between states $i$ and $j$ is calculated as the probability that a randomly selected pair of users from $i$ and $j$ respectively are Facebook friends (the original work~\cite{bailey2018social} had then scaled SCI scores for all geographical regions in the world to the range of 1 to 1 billion). Here, we determined the median SCI for pairs of states that are approximately $d$ distance apart where $d=\{0km, 100km, 200km...\}$ (distance between 2 states were measured using their geographic centers). As shown in Figure~\ref{fig:geoprob2}, we observed that SCI dropped sharply when $i\neq j$. In other words, most Facebook friends are from the same state. Additionally, the geographical segregation is more prominent on Facebook compared to Reddit. For instance, the SCI index dropped by a factor of $208$ from $d=0$ to $d=100km$. In comparison $Connectivity$ on Reddit only dropped by a factor of $20$.

\begin{figure}[ptb]
    \centering
    \includegraphics[width=0.4\linewidth]{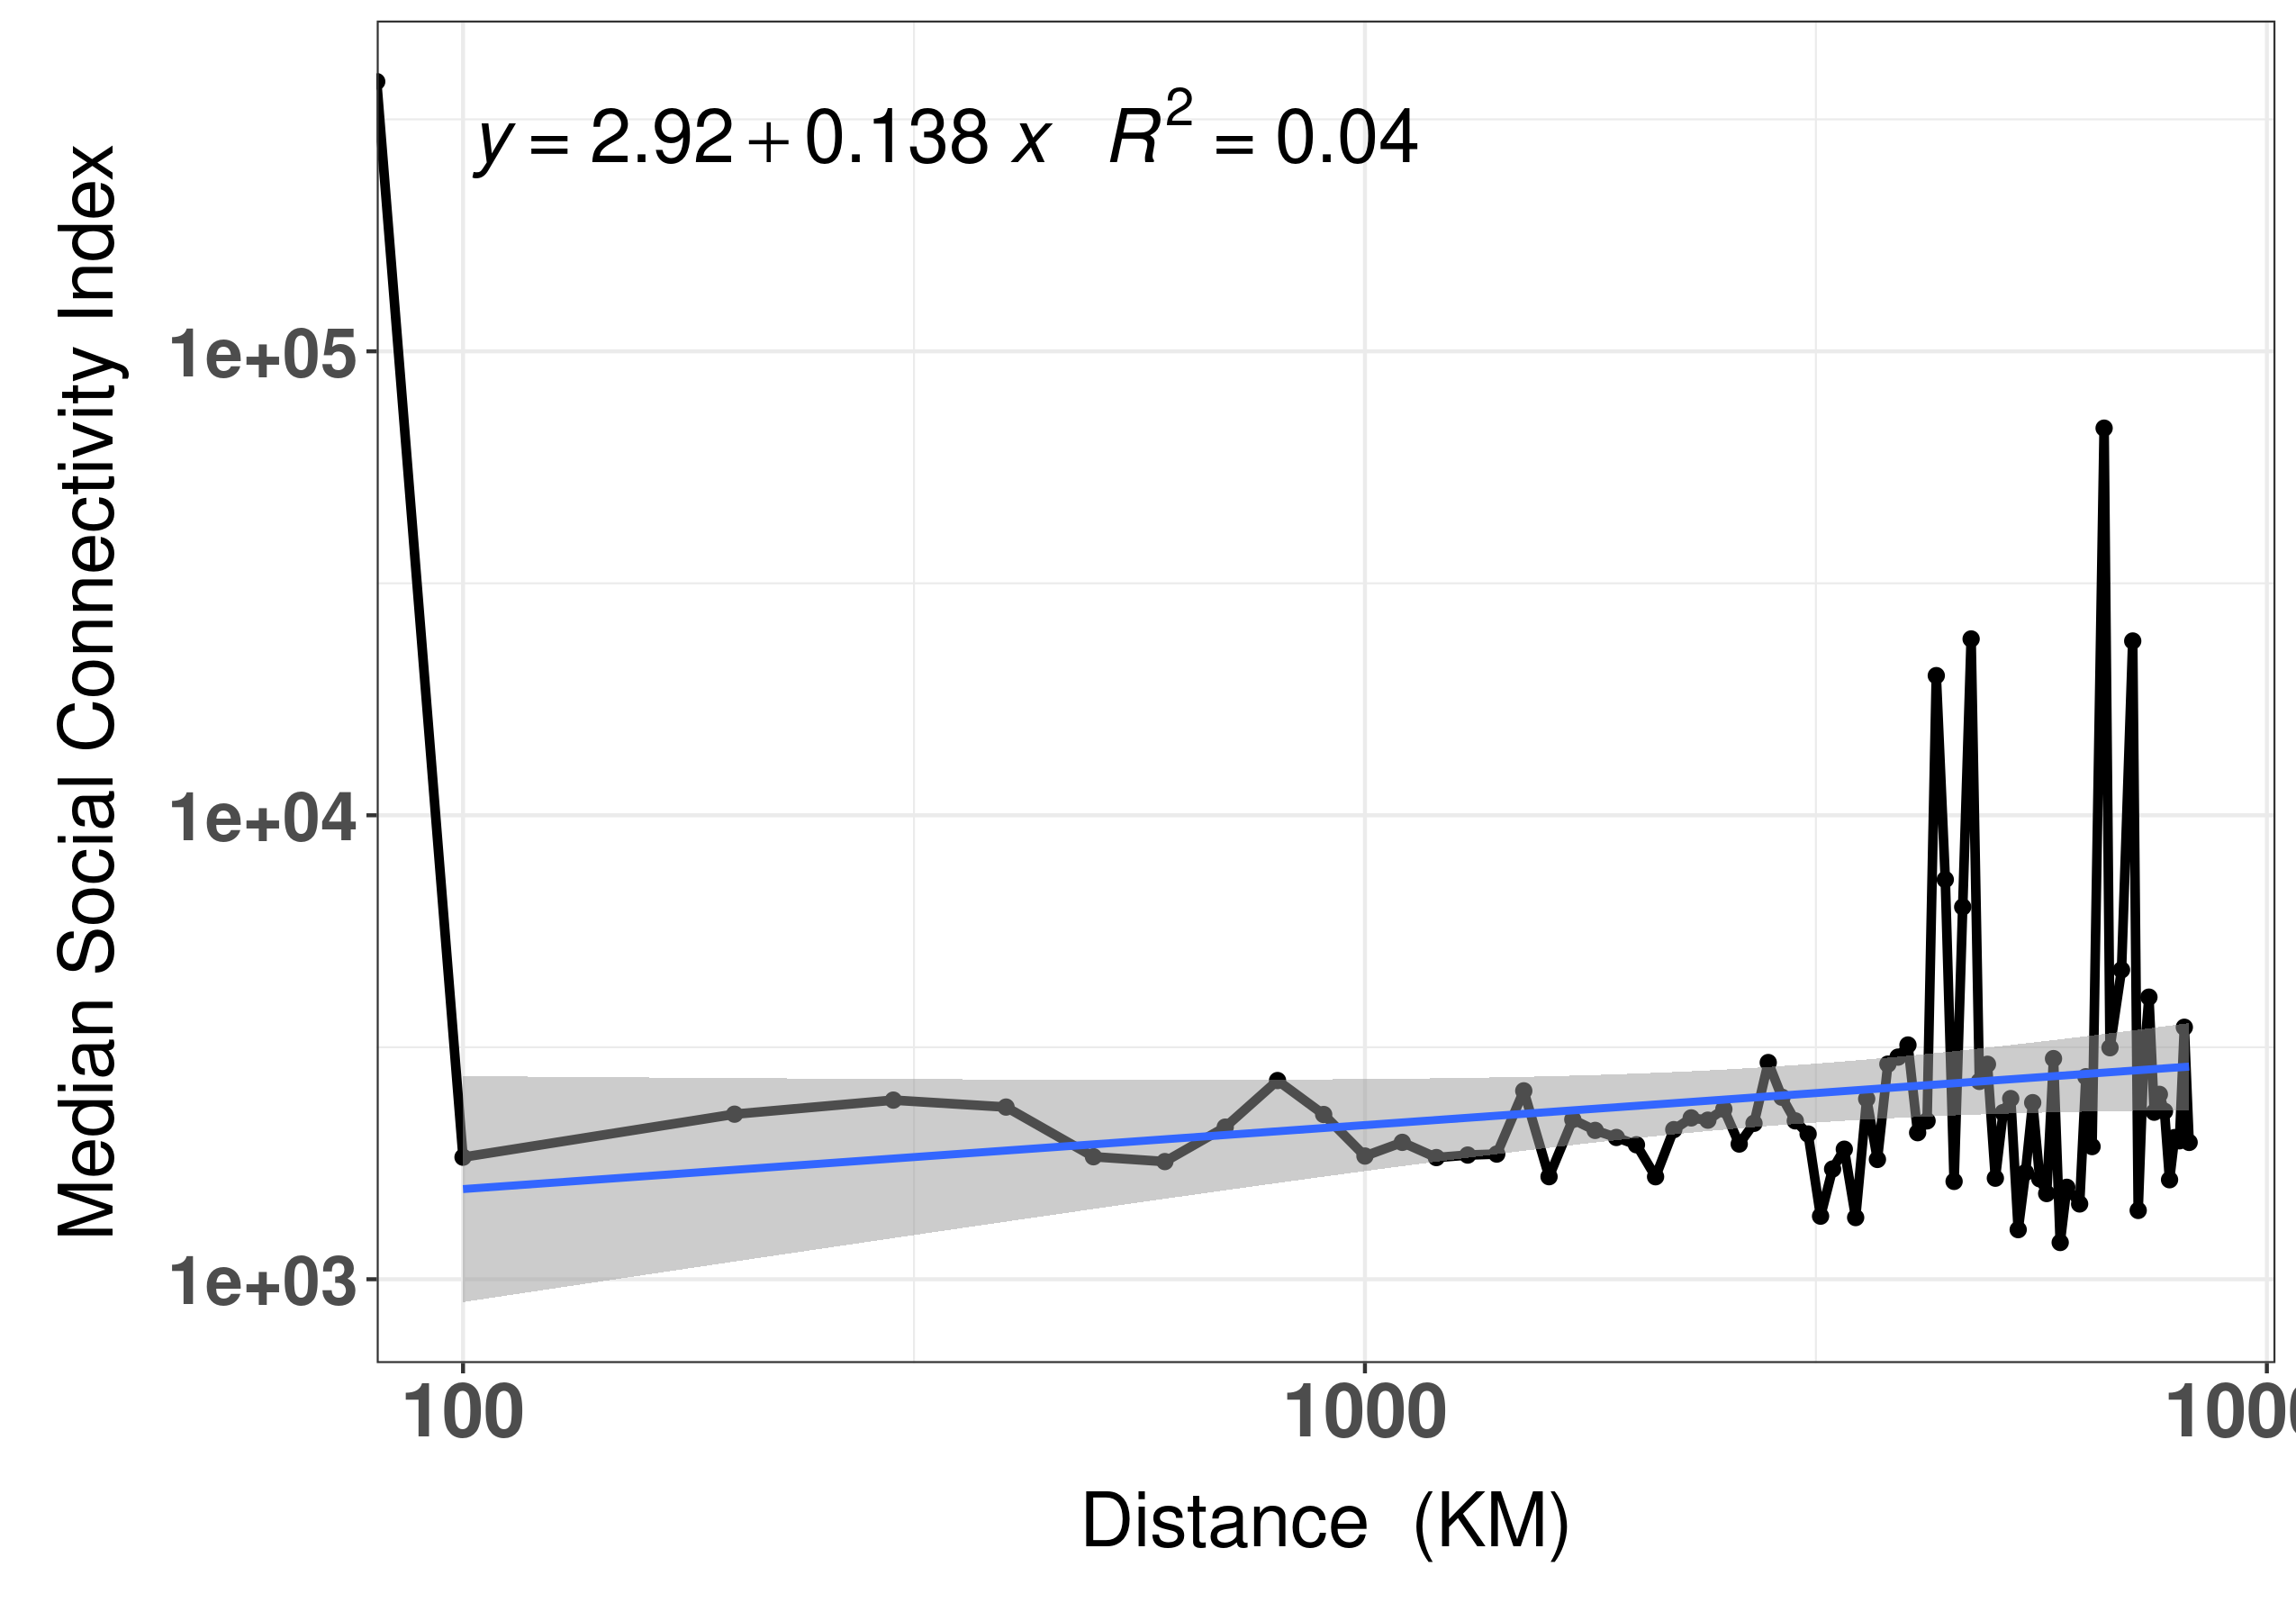}
    \caption{Facebook Social Connectivity Index. The x-axis denotes the geographical distance and the y-axis is the median social connectivity index between regions that's $x$ distance apart~\cite{bailey2018social}. We observed a similar, albeit much more extreme, pattern of geographical segregation.}
    \label{fig:geoprob2}
\end{figure}

\subsection*{The Big Sort}
Additional analyses in this section demonstrated that our initial findings are robust.

\subsubsection*{Types of state-level attributes} 
We included separate regression models fitted with only socioeconomic variables (Table~\ref{tab:circulation_partial_socio}) or political variables (Table~\ref{tab:circulation_partial_pol}). We then compared the $R^2$ of these models with the models fitted with only personality and cultural variables (Table 3 in the main text). We observed that the models fitted with only personality and cultural variables had the highest $R^2$ than models fitted with only socioeconomic or political variables. Next, by comparing the full models (Table 3 in the main text) and models that included all variables except for personality and culture (Table~\ref{tab:circulation_partial_other}),  we also saw that adding personality and cultural variables increased the $R^2$ values by 0.1 to 0.2. Both analyses demonstrated that personality and cultural factor are strong indicators of circulation.
\begin{table}[!t] \centering \small
\caption{Regression Results for Circulation Using Only Socioeconomic Attributes. We saw that states with a higher average income had higher-than-expected circulation for all news types. More importantly, the variance explained by socioeconomic conditions was comparable or slightly lower than the variance explained by personality and cultural factors (see Table 3).}
  \label{tab:circulation_partial_socio} 
\begin{tabular}{@{\extracolsep{5pt}}lccc} 
\\[-1.8ex]\hline 
\hline \\[-1.8ex] 
 & \multicolumn{3}{c}{\textit{Dependent variable: circulation}} \\ 
\cline{2-4} 
 & reputable & lowcred & fake \\ 
\\[-1.8ex] & (1) & (2) & (3)\\ 
\hline \\[-1.8ex] 
 no\_highschool &  & 0.035 (0.022) &  \\ 
  gdp & 0.071$^{***}$ (0.017) & 0.066$^{***}$ (0.017) & 0.049$^{***}$ (0.016) \\ 
  density & $-$0.024 (0.017) &  &  \\ 
  minority &  & $-$0.034 (0.022) &  \\ 
  Constant & $-$0.006 (0.013) & $-$0.002 (0.014) & 0.001 (0.016) \\ 
 \hline \\[-1.8ex] 
Observations & 48 & 48 & 48 \\ 
R$^{2}$ & 0.319 & 0.256 & 0.170 \\ 
Adjusted R$^{2}$ & 0.289 & 0.206 & 0.152 \\ 
Residual Std. Error & 0.087 (df = 45) & 0.097 (df = 44) & 0.108 (df = 46) \\ 
F Statistic & 10.530$^{***}$ (df = 2; 45) & 5.053$^{***}$ (df = 3; 44) & 9.451$^{***}$ (df = 1; 46) \\ 
\hline 
\hline \\[-1.8ex] 
\textit{Note:}  & \multicolumn{3}{r}{$^{*}$p$<$0.1; $^{**}$p$<$0.05; $^{***}$p$<$0.01} \\ 
\end{tabular} 
\end{table} 
% Table created by stargazer v.5.2.2 by Marek Hlavac, Harvard University. E-mail: hlavac at fas.harvard.edu
% Date and time: Thu, Aug 12, 2021 - 09:38:48 PM
\begin{table}[!t] \centering \small
\caption{Regression Results for Circulation Using Only Political Attributes. We saw that Republican-leaning and politically disengaged states had lower-than-expected circulation. More importantly, we also observed that the variance explained by political attributes was much lower than the variance explained by personality and cultural factors (see Table 3 in the main text).} 
  \label{tab:circulation_partial_pol}  
\begin{tabular}{@{\extracolsep{5pt}}lccc} 
\\[-1.8ex]\hline 
\hline \\[-1.8ex] 
 & \multicolumn{3}{c}{\textit{Dependent variable: circulation}} \\ 
\cline{2-4} 
 & reputable & lowcred & fake \\ 
\\[-1.8ex] & (1) & (2) & (3)\\ 
\hline \\[-1.8ex] 
 republican & $-$0.043$^{***}$ (0.013) & $-$0.040$^{**}$ (0.015) & $-$0.032$^{*}$ (0.017) \\ 
  political & 0.026$^{*}$ (0.013) &  &  \\ 
  Constant & $-$0.006 (0.013) & $-$0.002 (0.015) & 0.001 (0.016) \\ 
 \hline \\[-1.8ex] 
Observations & 48 & 48 & 48 \\ 
R$^{2}$ & 0.246 & 0.131 & 0.075 \\ 
Adjusted R$^{2}$ & 0.213 & 0.112 & 0.055 \\ 
Residual Std. Error & 0.092 (df = 45) & 0.103 (df = 46) & 0.114 (df = 46) \\ 
F Statistic & 7.342$^{***}$ (df = 2; 45) & 6.939$^{**}$ (df = 1; 46) & 3.754$^{*}$ (df = 1; 46) \\ 
\hline 
\hline \\[-1.8ex] 
\textit{Note:}  & \multicolumn{3}{r}{$^{*}$p$<$0.1; $^{**}$p$<$0.05; $^{***}$p$<$0.01} \\ 
\end{tabular} 
\end{table} 
% Table created by stargazer v.5.2.2 by Marek Hlavac, Harvard University. E-mail: hlavac at fas.harvard.edu
% Date and time: Thu, Aug 12, 2021 - 09:39:48 PM
\begin{table}[!t] \centering \small
\caption{Regression Results for Circulation Using All Attributes Except for Personality and Culture. We saw that personality and cultural factors explained any additional 10\% to 20\% of the variance. As an example, the full model for reputable news using all variables had adjusted $R^2=0.45$. Here, we saw that the same model excluding personality and culture only had adjusted $R^2=0.338$ (a difference of approximately 0.11).}
  \label{tab:circulation_partial_other} 
\begin{tabular}{@{\extracolsep{5pt}}lccc} 
\\[-1.8ex]\hline 
\hline \\[-1.8ex] 
 & \multicolumn{3}{c}{\textit{Dependent variable: circulation}} \\ 
\cline{2-4} 
 & reputable & lowcred & fake \\ 
\\[-1.8ex] & (1) & (2) & (3)\\ 
\hline \\[-1.8ex] 
 no\_highschool &  & 0.033 (0.022) &  \\ 
  gdp & 0.062$^{***}$ (0.017) & 0.072$^{***}$ (0.022) & 0.049$^{***}$ (0.016) \\ 
  minority &  & $-$0.031 (0.022) &  \\ 
  density & $-$0.038$^{**}$ (0.017) & $-$0.033 (0.020) &  \\ 
  republican & $-$0.033$^{**}$ (0.016) & $-$0.025 (0.019) &  \\ 
  Constant & $-$0.006 (0.012) & $-$0.002 (0.014) & 0.001 (0.016) \\ 
 \hline \\[-1.8ex] 
Observations & 48 & 48 & 48 \\ 
R$^{2}$ & 0.380 & 0.313 & 0.170 \\ 
Adjusted R$^{2}$ & 0.338 & 0.231 & 0.152 \\ 
Residual Std. Error & 0.084 (df = 44) & 0.096 (df = 42) & 0.108 (df = 46) \\ 
F Statistic & 9.003$^{***}$ (df = 3; 44) & 3.831$^{***}$ (df = 5; 42) & 9.451$^{***}$ (df = 1; 46) \\ 
\hline 
\hline \\[-1.8ex] 
\textit{Note:}  & \multicolumn{3}{r}{$^{*}$p$<$0.1; $^{**}$p$<$0.05; $^{***}$p$<$0.01} \\ 
\end{tabular} 
\end{table} 

\subsubsection*{Normalized Circulation}
In this section, , we redefined $Circulation(s, i)$ as the average number of comments containing URLs to news type $s$ posted by Reddit users from state $i$. We then reran Equation 1 from the main text. Results are summarized on Table~\ref{tab:circulation_ave}. As shown, personality and cultural variables were still strongly indicative of circulation for all news types. For instance, the reputable news circulation model that included only personality and cultural variables had an adjusted $R^2$ of 0.32. In comparison, the full model's $R^2$ was 0.57. Furthermore, We again saw that {\it conscientiousness} was significantly and negatively correlated with the circulation of all news types. Additionally, the coefficient for {\it cultural tightness} is negative but not significant.
% Table created by stargazer v.5.2.2 by Marek Hlavac, Harvard University. E-mail: hlavac at fas.harvard.edu
% Date and time: Thu, Aug 12, 2021 - 09:43:06 PM
\begin{table}[!t] \centering \scriptsize
    \caption{Regression Results for Circulation Fraction. Here, the dependent variable was calculated as the average number of comments posted by users from a given state for each news type. We observed comparable results: personality and culture were strong indicators of circulation.} 
  \label{tab:circulation_ave} 
\begin{tabular}{@{\extracolsep{-5pt}}lp{2.2cm} p{2.2cm} p{2.2cm} p{2.2cm} p{2.2cm} p{2.2cm}} 
\\[-1.8ex]\hline 
\hline \\[-1.8ex] 
 & \multicolumn{6}{c}{\textit{Dependent variable: circulation fraction}} \\ 
\cline{2-7} 
 & reputable mod (personality and culture) & reputable mod (complete) & lowcred mod (personality and culture) & lowcred mod (complete) & fake mod (personality and culture) & fake mod (complete) \\ 
\\[-1.8ex] & (1) & (2) & (3) & (4) & (5) & (6)\\ 
\hline \\[-1.8ex] 
 extraversion & 0.208$^{*}$ (0.123) &  & 0.013 (0.009) &  & 0.004$^{*}$ (0.002) &  \\ 
  agreeableness & 0.283$^{*}$ (0.143) & 0.239$^{**}$ (0.118) & 0.019$^{*}$ (0.010) & 0.021$^{**}$ (0.009) & 0.004$^{*}$ (0.002) & 0.005$^{**}$ (0.002) \\ 
  conscientiousness & $-$0.398$^{**}$ (0.153) & $-$0.349$^{***}$ (0.120) & $-$0.029$^{**}$ (0.011) & $-$0.024$^{**}$ (0.009) & $-$0.006$^{**}$ (0.003) & $-$0.004$^{*}$ (0.002) \\ 
  openness & 0.329$^{**}$ (0.133) &  & 0.018$^{*}$ (0.010) &  & 0.004$^{*}$ (0.002) & $-$0.003 (0.002) \\ 
  cultural\_tightness & $-$0.306$^{**}$ (0.136) & $-$0.344$^{***}$ (0.123) & $-$0.017 (0.010) & $-$0.019$^{**}$ (0.009) & $-$0.003 (0.002) & $-$0.006$^{**}$ (0.002) \\ 
  no\_highschool &  & 0.294$^{**}$ (0.122) &  & 0.032$^{***}$ (0.008) &  & 0.009$^{***}$ (0.002) \\ 
  population &  & 0.267$^{**}$ (0.122) &  &  &  &  \\ 
  gdp &  & 0.373$^{**}$ (0.160) &  & 0.032$^{***}$ (0.011) &  & 0.007$^{***}$ (0.002) \\ 
  density &  & $-$0.229$^{*}$ (0.124) &  & $-$0.016 (0.010) &  &  \\ 
  Constant & 2.676$^{***}$ (0.107) & 2.676$^{***}$ (0.085) & 0.194$^{***}$ (0.008) & 0.194$^{***}$ (0.007) & 0.042$^{***}$ (0.002) & 0.042$^{***}$ (0.001) \\ 
 \hline \\[-1.8ex] 
Observations & 48 & 48 & 48 & 48 & 48 & 48 \\ 
R$^{2}$ & 0.396 & 0.638 & 0.311 & 0.523 & 0.275 & 0.496 \\ 
Adjusted R$^{2}$ & 0.324 & 0.574 & 0.229 & 0.453 & 0.189 & 0.423 \\ 
Residual Std. Error & 0.740 (df = 42) & 0.587 (df = 40) & 0.054 (df = 42) & 0.045 (df = 41) & 0.012 (df = 42) & 0.010 (df = 41) \\ 
F Statistic & 5.515$^{***}$ (df = 5; 42) & 10.056$^{***}$ (df = 7; 40) & 3.797$^{***}$ (df = 5; 42) & 7.478$^{***}$ (df = 6; 41) & 3.187$^{**}$ (df = 5; 42) & 6.735$^{***}$ (df = 6; 41) \\ 
\hline 
\hline \\[-1.8ex] 
\textit{Note:}  & \multicolumn{6}{r}{$^{*}$p$<$0.1; $^{**}$p$<$0.05; $^{***}$p$<$0.01} \\ 
\end{tabular} 
\end{table} 

\subsubsection*{Satirical News}
Circulation analysis for satirical news are summarized in Table~\ref{tab:circulation_satire}. We included 3 partial models each only included a category of state-level attributes and a 4th full model which contained all explanatory variables. Note that all models were fitted with stepAIC. We again saw that the difference in $R^2$ was small for the model that included only the personality and cultural variables and the full model (a difference of $0.372-0.342=0.03$). Additionally, {\it cultural tightness} is significantly and negatively correlated with circulation of satirical news. Further, the coefficient for {\it conscientiousness} was not significant, though its directionality remained negative ($\beta<0$).
% Table created by stargazer v.5.2.2 by Marek Hlavac, Harvard University. E-mail: hlavac at fas.harvard.edu
% Date and time: Thu, Aug 12, 2021 - 10:39:43 PM
\begin{table}[!t] \centering \small
\caption{Circulation of Satirical News. We again saw that that personality and cultural factors (specifically, {\it conscientiousness} and {\it cultural tightness}) alone explained a considerable portion of the variance.} 
  \label{tab:circulation_satire} 
\begin{tabular}{@{\extracolsep{5pt}}lcccc} 
\\[-1.8ex]\hline 
\hline \\[-1.8ex] 
 & \multicolumn{4}{c}{\textit{Dependent variable: circulation}} \\ 
\cline{2-5} 
 & personality and culture & socioeconomic & political & complete \\ 
\\[-1.8ex] & (1) & (2) & (3) & (4)\\ 
\hline \\[-1.8ex] 
 conscientiousness & $-$0.047$^{**}$ (0.019) &  &  &  \\ 
  agreeableness &  &  &  & 0.033 (0.021) \\ 
  neuroticism &  &  &  & 0.048$^{**}$ (0.019) \\ 
  cultural\_tightness & $-$0.054$^{***}$ (0.019) &  &  & $-$0.050$^{**}$ (0.021) \\ 
  gdp &  & 0.091$^{***}$ (0.017) &  & 0.067$^{***}$ (0.021) \\ 
  minority &  & $-$0.042$^{**}$ (0.017) &  &  \\ 
  republican &  &  & $-$0.051$^{**}$ (0.019) &  \\ 
  political &  &  & 0.035$^{*}$ (0.019) &  \\ 
  Constant & $-$0.008 (0.017) & $-$0.008 (0.016) & $-$0.008 (0.019) & $-$0.008 (0.016) \\ 
 \hline \\[-1.8ex] 
Observations & 48 & 48 & 48 & 48 \\ 
R$^{2}$ & 0.370 & 0.398 & 0.193 & 0.455 \\ 
Adjusted R$^{2}$ & 0.342 & 0.372 & 0.157 & 0.405 \\ 
Residual Std. Error & 0.116 (df = 45) & 0.113 (df = 45) & 0.131 (df = 45) & 0.110 (df = 43) \\ 
F Statistic & 13.229$^{***}$ (df = 2; 45) & 14.897$^{***}$ (df = 2; 45) & 5.369$^{***}$ (df = 2; 45) & 8.984$^{***}$ (df = 4; 43) \\ 
\hline 
\hline \\[-1.8ex] 
\textit{Note:}  & \multicolumn{4}{r}{$^{*}$p$<$0.1; $^{**}$p$<$0.05; $^{***}$p$<$0.01} \\ 
\end{tabular} 
\end{table} .
